# Supplementary material for: Signatures of Light Massive Relics on nonlinear structure formation
Source: arXiv:2202.09840 source file (2022-02-20)
Supplement: Supplementary file 1 [file appendix_extra.tex]

\begin{figure}[htp!]
\centering
\includegraphics[scale=0.49]{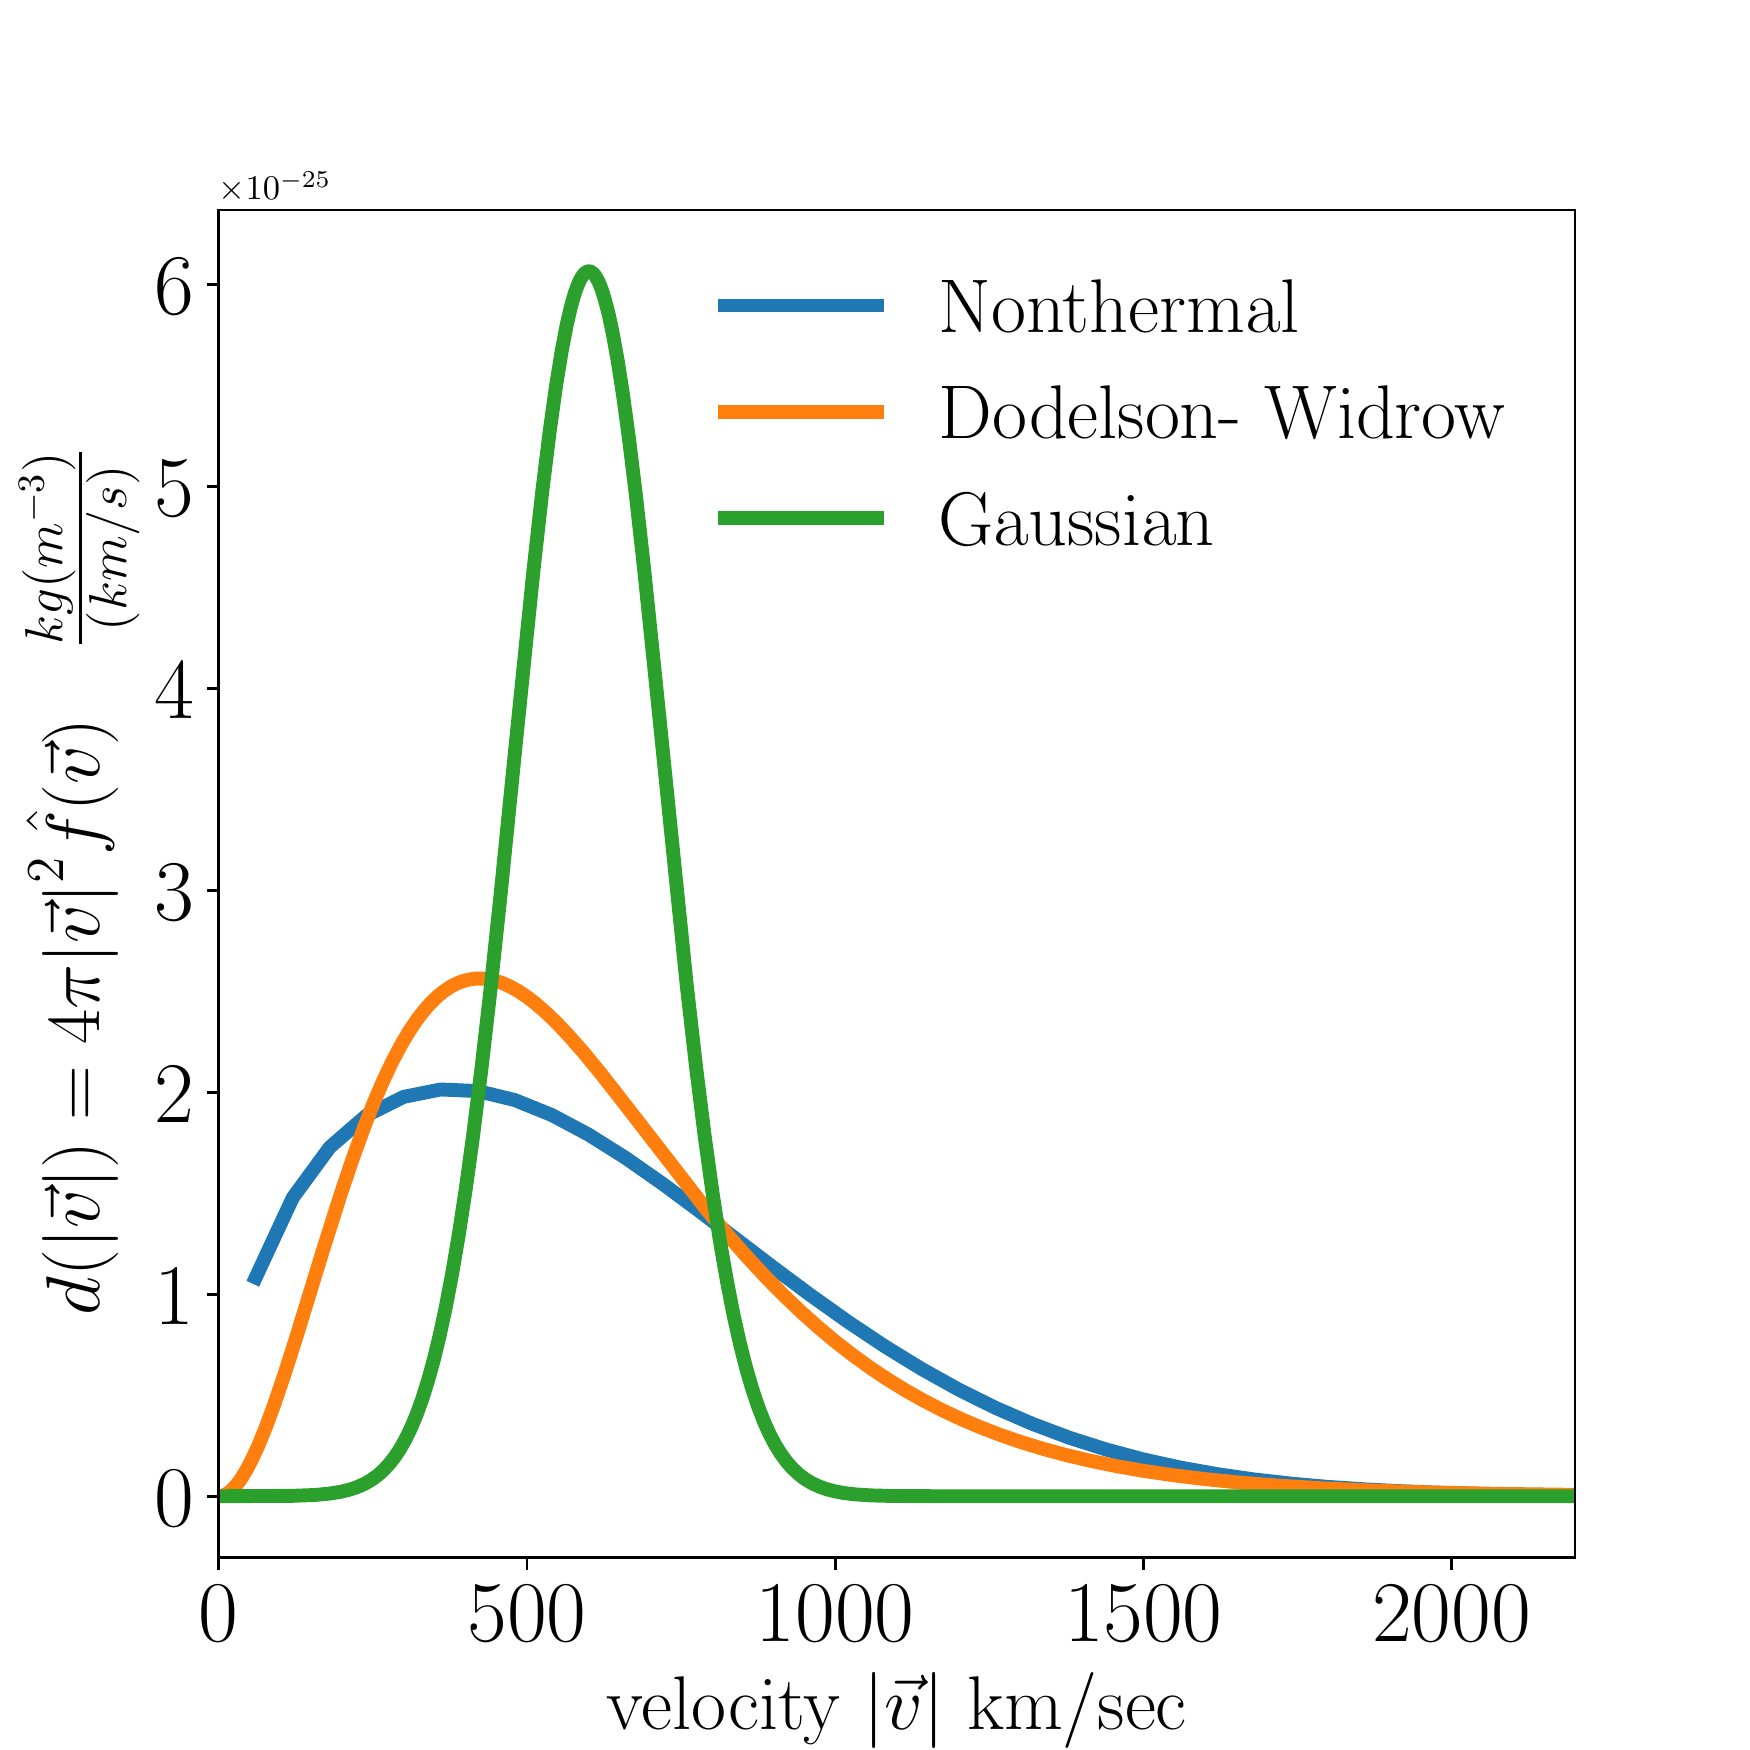}
\includegraphics[scale=0.345]{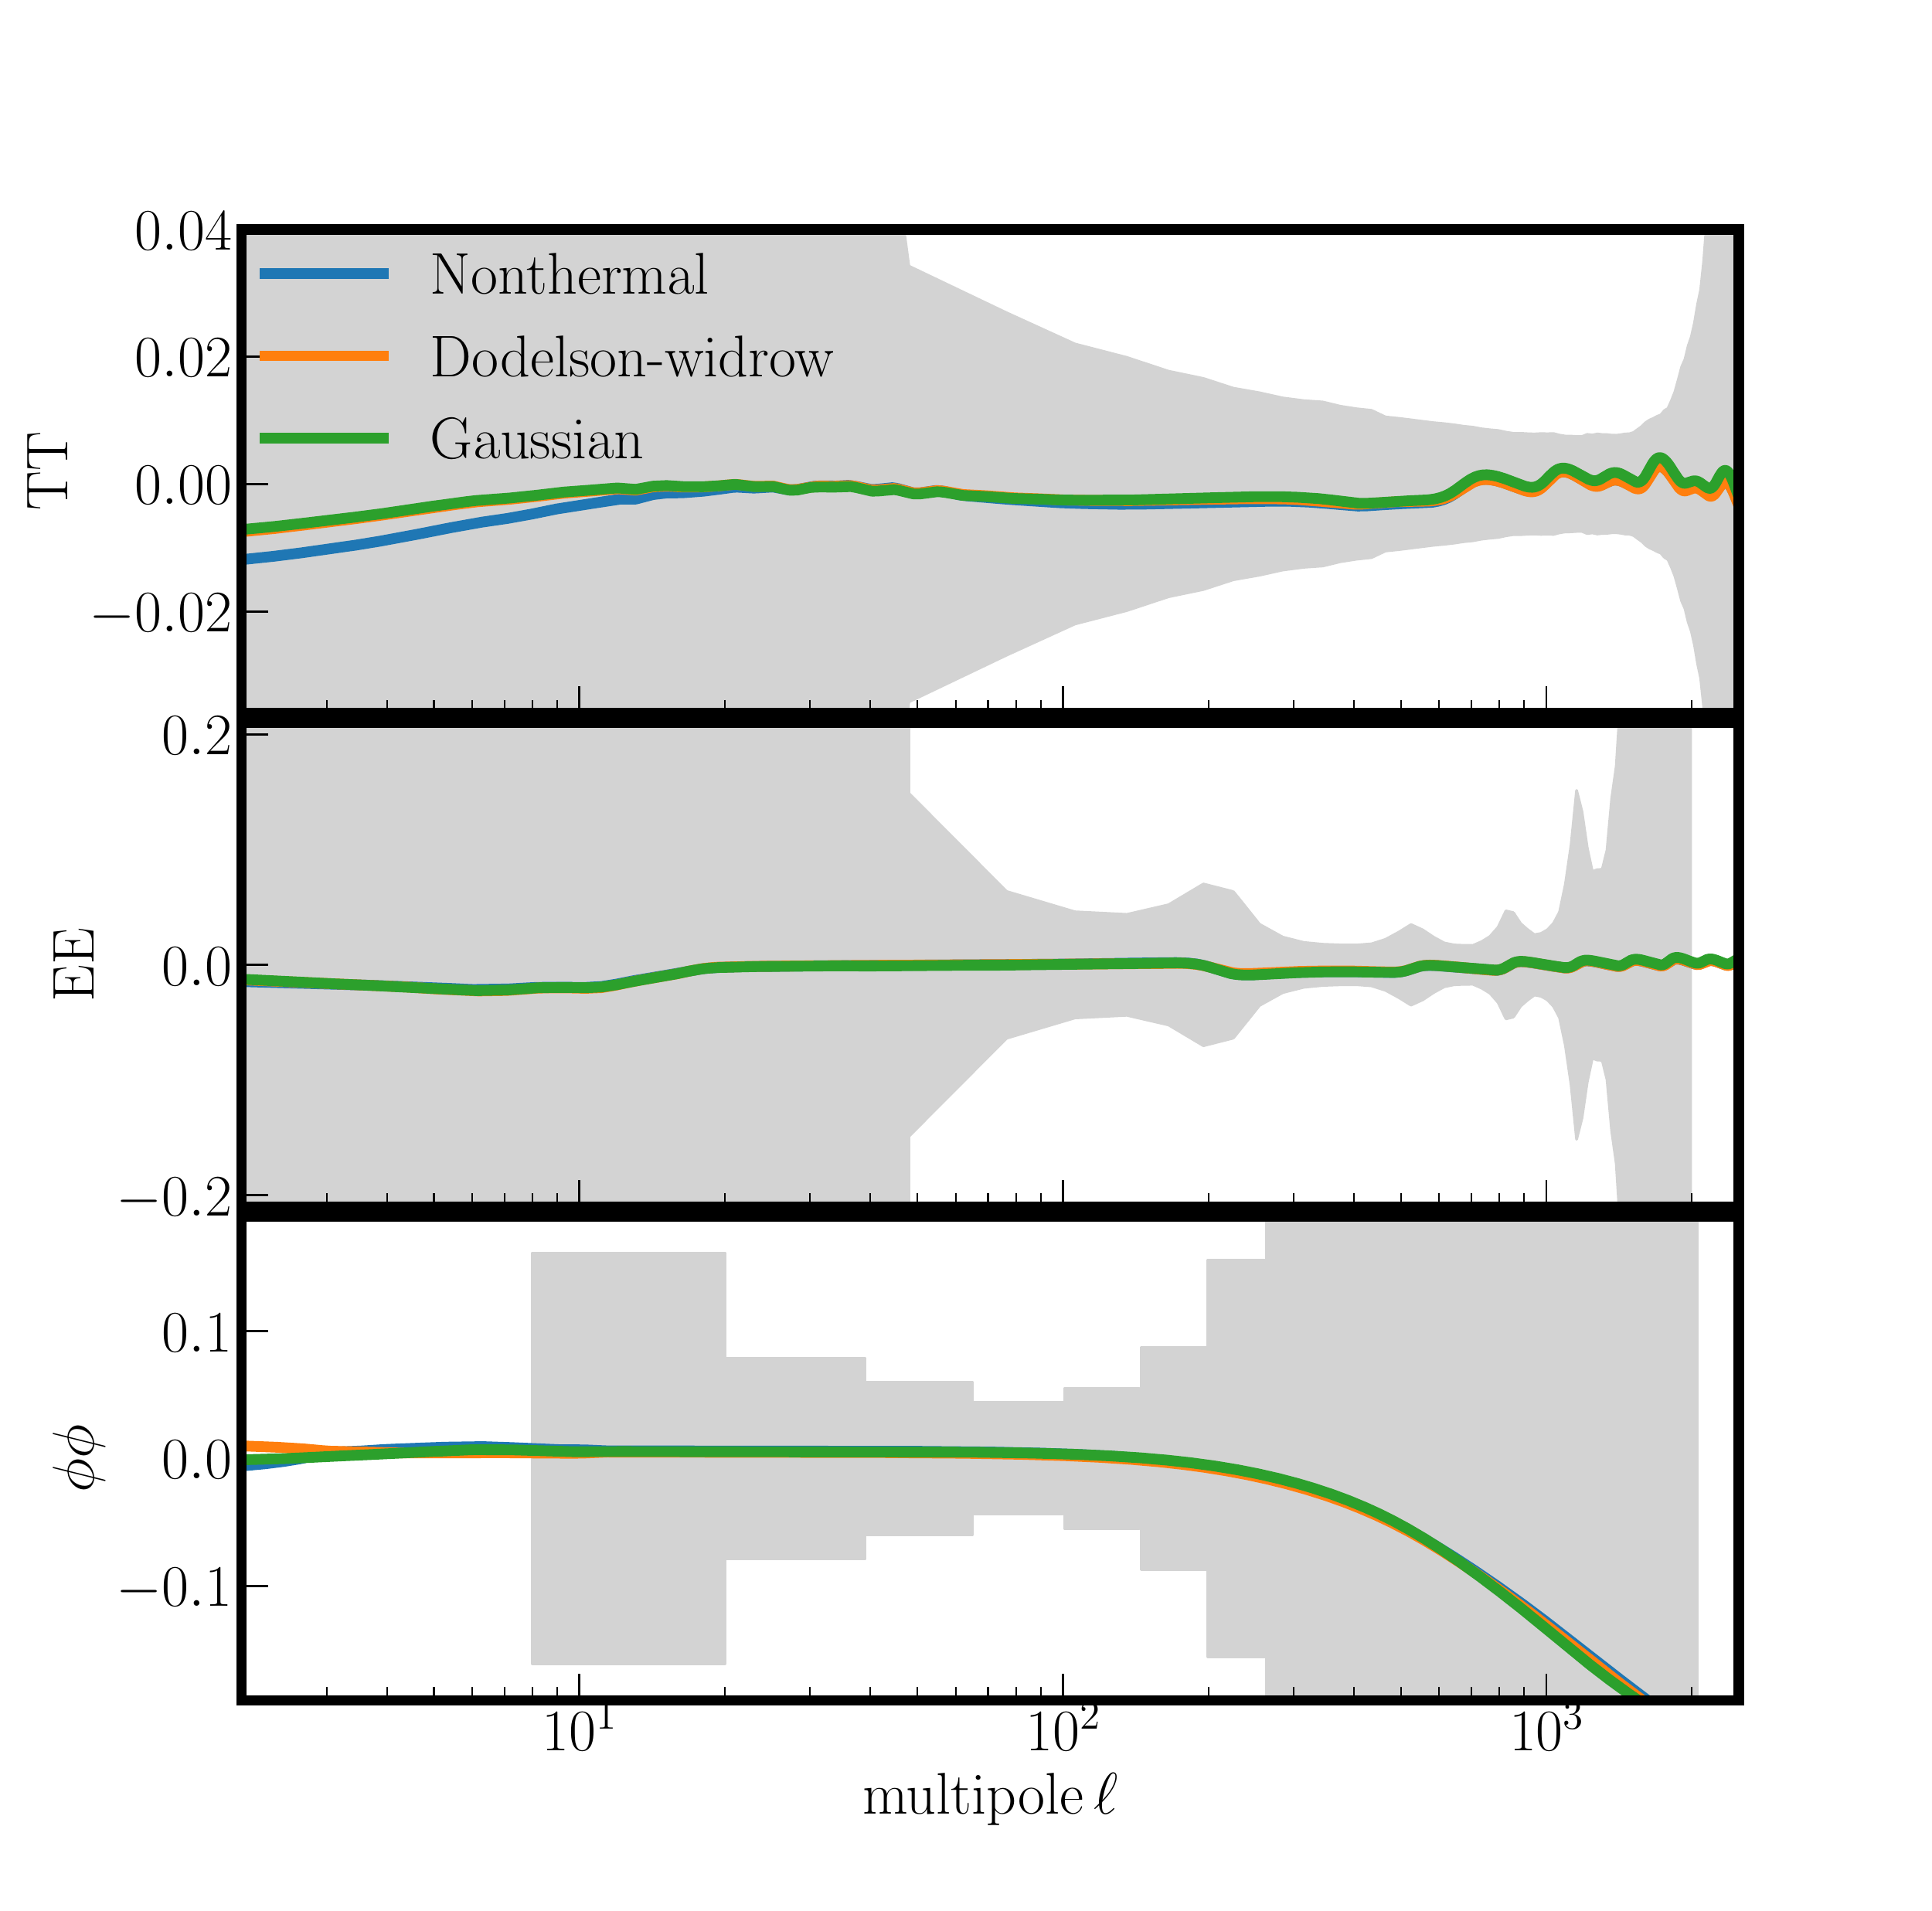}
\caption{The  plot shows velocity distribution of Dodelson widrow and Nonthermal distribution from moduli decay  Gaussian distribution and thermal with a different temperature compare to standard model. All four distributions are corresponding to same $\Delta N_{\rm eff}=0.034$ and same $ms_{\rm eff}=0.90$. \ab{To hammer home the point of indistinguishability at CMB level, can we plot the Planck residuals for all three as a right panel? Also, just for consistency, extend the blue curve to 0, since you are doing it for the other two.
XXX  label for the y-axis consistent with the plot in the main text}} 
%\label{fig:psd} 
\end{figure}

   LIMRs with negligible interactions are completely characterised by their distribution functions and their mass. In the linear theory, the physics is sensitive only to the first two moments of their distribution functions (see e.g \citep{Acero:2008rh}) and all observables are determined by two parameters. The first of these is the effective mass parameter $(m_{\rm eff})$, a measure of the contribution of the sterile particles to the present day energy density
\begin{equation}
\frac{m_{\rm eff}}{94.05 {\rm eV}} = \left[
{{m_{\rm sp}} \int \!\! dp \,\, p^2 f(p)} 
\right] \times \left[\frac{h^2}{\rho_c^0}\right],
\end{equation}  
 where $m_{\rm sp}$  is the physical mass of sterile particle and $\rho_c^0$ the total energy density of the universe today. The second parameter is
$\Delta N_{\rm eff}$, which measures the effective number of neutrino-like relativistic degrees of freedom at the time of neutrino decoupling
\begin{equation}
\Delta N_{\rm eff} \equiv \frac{\rho_s^{\rm rel}}{\rho_\nu}
= \left[
{ \int \!\! dp \,\, p^3 f(p)} 
\right] /
\left[{\frac{7}{8} \frac{\pi^2}{15}
{T_\nu}^4} \right]  
\end{equation}
with $T_\nu \equiv (4/11)^{1/3} T_{\rm cmb}$, the present day temperature of the cosmic neutrino background.

   The fact that the linear cosmology  just depends  on just two parameters implies that the CMB and linear matter power spectra are not effective probes of
the distribution function of LiMRs. In this appendix we will see that this situation changes when one considers non-linear effects. To explicitly see this
we will consider two other LiMR distribution functions which have the same values of $m_{\rm eff}$ and $\Delta N_{\rm eff}$ as the distribution function in 
the main text and obtain the non-linear cosmologies for these.  We will find that XXX the non-linear cosmologies are distinct and can be distinguished by 
photometric surveys.

  The LiMR distribution functions we will consider are 
\begin{itemize}
\item \underline{\it{The  Dodelson-Widrow distribution \cite{PhysRevLett.72.17}}}: The momentum distribution takes the form
$$
f(p)=\frac{\chi}{\rm exp(p/T_{\nu})+1} \, 
$$
where $\chi$ is a parameter. The model has the  same values of $\Delta N_{\rm eff}$ and $m_{\rm eff}$ as the  model in the main text if $\chi=0.034$ and $m_s=26.43\rm{eV}$ \cite{Das:2021pof}.

 \item \underline{\it{ A Gaussian  distribution \cite{Cuoco:2005qr}}}: The momentum distribution function takes the form
 $$
 f(\vec{p}) = N { T^{3}_{\nu} \over |\vec{p}|^2 } { \rm{exp} }\left(  -  \left( { ({|\vec{p}|   - p_0})^2 \over 2 \sigma^2  }\right)  \right) \,
 $$
 XXX RAVI: what is N
 where $p_0$, $\sigma$ are parameters. The model has the  same values of $\Delta N_{\rm eff}$ and $m_{\rm eff}$ as the model in the main text for $p_0=0.01957T_{\nu}$, $\sigma=\frac{p_0}{5}$ and $m_{\rm sp}=0.1644 \rm{eV}$.
\end{itemize}
 The matching of the effective parameters implies that the models are indistinguishable at the linear level. For completeness, we have computed the Planck residuals for residuals for the three models making use of CLASS. These
are exhibited in figure xxx. As expected the models are indistinguishable.

  Now, let us turn to the non-linear cosmologies. The first step is to obtain the mass distribution functions at $z=99$. These are easily computed from their momentum distribution functions.
  We exhibit them for the three models in figure \ref{fig:psd}.

MATERIAL FROm SEC 2, THIS SHOULD VANISH (keeping it here just in case we need something)

  The model has the  same values of $\Delta N_{\rm eff}$ and $m_{\rm eff}$ as the model in the main text for

The best fit values for the model parameters   were found be
. We will use these values to define the LiMR model that we explore in the rest of the paper.
 
To exhibit the main features of the linear cosmology of model, we present some plots summarising the results of \cite{Das:2021pof}. CMB residuals with respect to the best-fit $\Lambda$CDM model along with  \planck 2018 \cite{Planck:2018nkj} error bars are shown 
in Fig \ref{fig:cl}. It is clear from the plots of $C_l^{TT}$, $C_l^{EE}$, and $C_l^{\phi\phi}$ that the best-fit LiMR model is almost indistinguishable from the $\Lambda$CDM model. In Fig. \ref{fig:pk_only}, we present aplot the residual of the $z=0$ linear theory power spectrum between the LiMR model and the \planck best-fit $\Lambda$CDM model. There is a suppression in the power for k above the free-streaming scale of the LiMR component i.e  $k > 0.1 h / \rm{Mpc}$ . This  suppression is responsible for alleviating the $\sigma_8$ (or $S_8$) XXX commit to one XXX tension.

In this appendix we will see that this situation changes when one considers non-linear effects. To explicitly see this
we will consider two other LiMR distribution functions which have the same values of $m_{\rm eff}$ and $\Delta N_{\rm eff}$ as the distribution function in 
the main text and obtain the non-linear cosmologies for these.  We will find that XXX the non-linear cosmologies are distinct and can be distinguished by 
photometric surveys.

  Now, let us turn to the non-linear cosmologies. The first step is to obtain the mass distribution functions at $z=99$. These are easily computed from their momentum distribution functions.
  We exhibit them for the three models in figure \ref{fig:psd}.

As mentioned in the introduction, to initiate the study of the impact of LiMRs on photometric observables 
on nonlinear scales,  we will focus
 on a particular model in the main text. In this section, we briefly describe the model and refer the reader to \cite{Bhattacharya:2020zap,Das:2021pof}
 for the details.  The LiMRs under consideration will have negligible interactions; they are completely characterised by their momentum distribution
 and mass. The momentum distribution of LiMRs is in turn determined by their production mechanism. We provide a brief summary below.

\begin{figure}[htp!]
\centering
\includegraphics[scale=0.35]{apj_cl.pdf}
\caption{ Residuals of CMB power spectra from \textit{Planck} corresponding for our nonthermal LiMR cosmology at its best fit values, $B_{\rm sp} = 0.0118$ and $m_{\rm sp} =38.62 \rm{eV}$. All residuals are calculated with respect to the best-fit $\Lambda$CDM model to the \planck data. The shaded grey regions represent the $1\sigma$ error bars from \planck. \ab{Can we shorten the legend? Maybe just ``residual"?}} 
\label{fig:cl} 
\end{figure}

\begin{figure}[htp!]
\centering
\includegraphics[scale=0.35]{apj_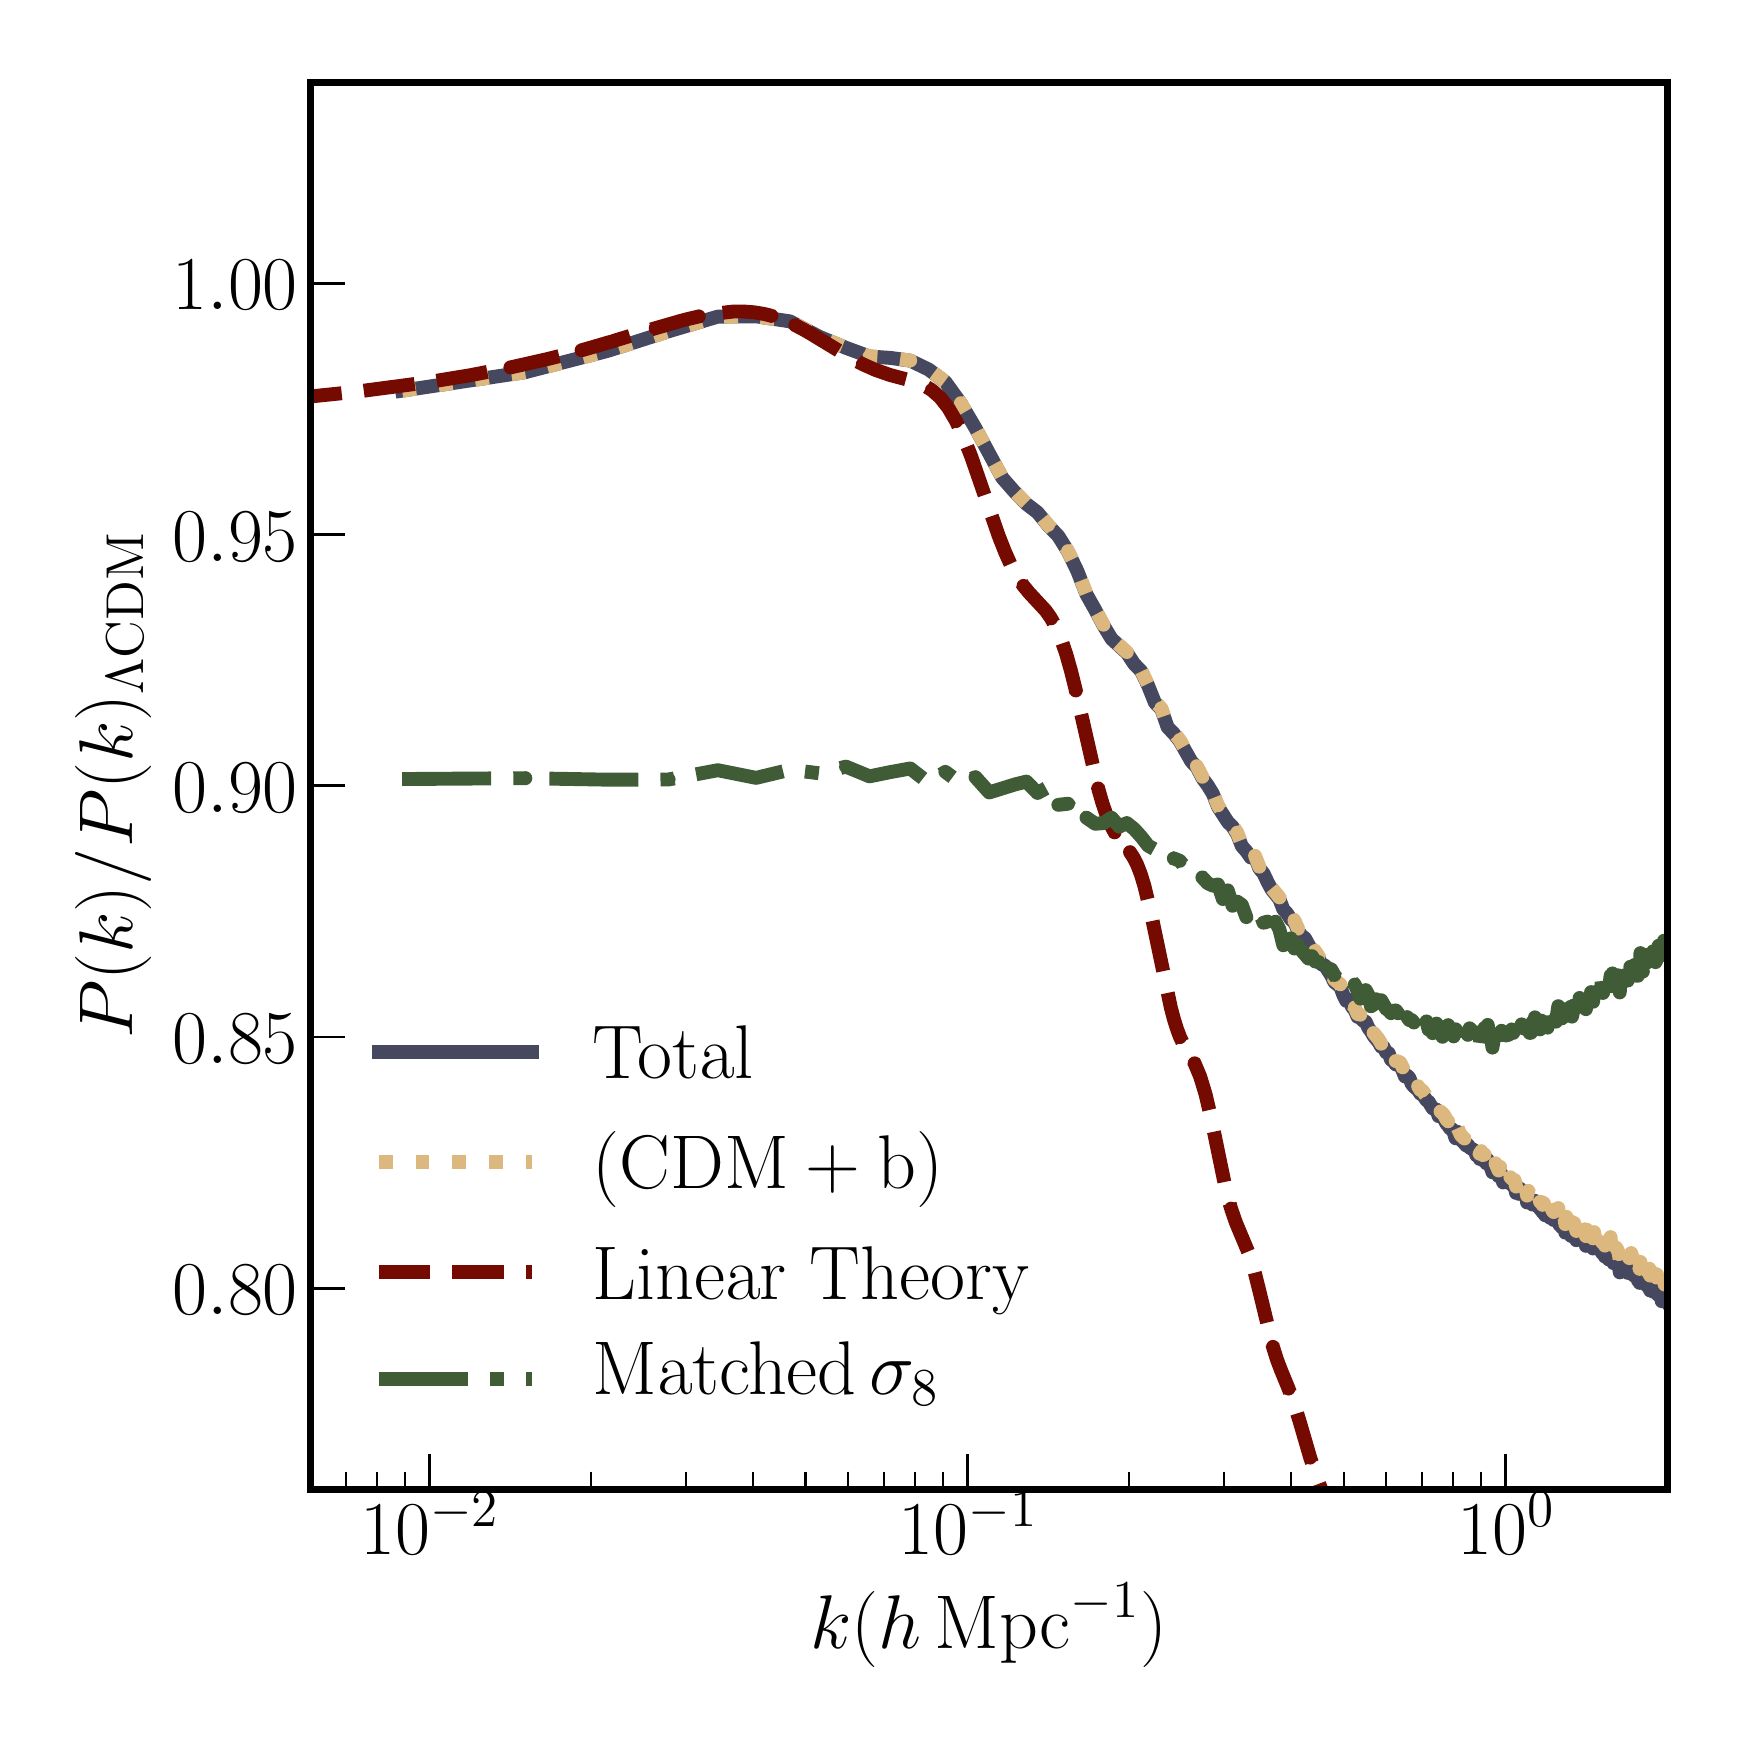}
\caption{ Residuals of Matter power spectra corresponding for our  Non-thermal distribution  at its best fit values, $B_{\rm sp} = 0.0118$ and $m_{\rm sp} =38.62 \rm{eV}$.  \ab{cut the x-axis on the left at $\sim 6 \times 10^{-3}\hmpc$? Also increase the font size on the axes labels.}} 
\label{fig:pk_only} 
\end{figure}
